# Supplementary material for: RecKG: Knowledge Graph for Recommender Systems
Source: arXiv:2501.03598 source file (2026-09-29)
Supplement: Supplementary file 1 [file A_appendix.tex]

% \appendix
% %Appendix A
% \section{Appendices}
% \subsection{The wide view of RecKG}
% % ====================================================================
% \begin{figure*}
%   \centering
%   \includegraphics[width=1.0\linewidth]{figures/semantic_web_style.png}
%   \caption{The wide view of integration of Yahoo!Movies to MovieLens in RecKG}
%   \label{fig:The wide view of integration of Yahoo!Movies to MovieLens in RecKG}
% \end{figure*}
% % ====================================================================






% % The rules about hierarchical headings discussed above for
% % the body of the article are different in the appendices.
% % In the \textbf{appendix} environment, the command
% % \textbf{section} is used to
% % indicate the start of each Appendix, with alphabetic order
% % designation (i.e., the first is A, the second B, etc.) and
% % a title (if you include one).  So, if you need
% % hierarchical structure
% % \textit{within} an Appendix, start with \textbf{subsection} as the
% % highest level. Here is an outline of the body of this
% % document in Appendix-appropriate form:
% % \subsection{Introduction}
% % \subsection{The Body of the Paper}
% % \subsection{Conclusions}
% % \subsection{References}
% % Generated by bibtex from your \texttt{.bib} file.  Run latex,
% % then bibtex, then latex twice (to resolve references)
% % to create the \texttt{.bbl} file.  Insert that \texttt{.bbl}
% % file into the \texttt{.tex} source file and comment out
% % the command \texttt{{\char'134}thebibliography}.
% % % This next section command marks the start of
% % % Appendix B, and does not continue the present hierarchy
% % \section{More Help for the Hardy}

% % Of course, reading the source code is always useful.  The file
% % \path{acmart.pdf} contains both the user guide and the commented
% % code.

% % % ACKNOWLEDGMENTS
% % % \begin{acks}
% % %   The authors would like to thank Dr. Yuhua Li for providing the
% % %   matlab code of  the \textit{BEPS} method. 

% % %   The authors would also like to thank the anonymous referees for
% % %   their valuable comments and helpful suggestions. The work is
% % %   supported by the \grantsponsor{GS501100001809}{National Natural
% % %     Science Foundation of
% % %     China}{http://dx.doi.org/10.13039/501100001809} under Grant
% % %   No.:~\grantnum{GS501100001809}{61273304}
% % %   and~\grantnum[http://www.nnsf.cn/youngscientsts]{GS501100001809}{Young
% % %     Scientsts' Support Program}.

% % % \end{acks}
